# Supplementary material for: A Graph Theory approach to assess nature's contribution to people at a global scale
Source: arXiv:2007.14308 source file (2021-02-15)
Supplement: Supplementary file 1 [file SI_FigA1_lowres.pdf]

1A)

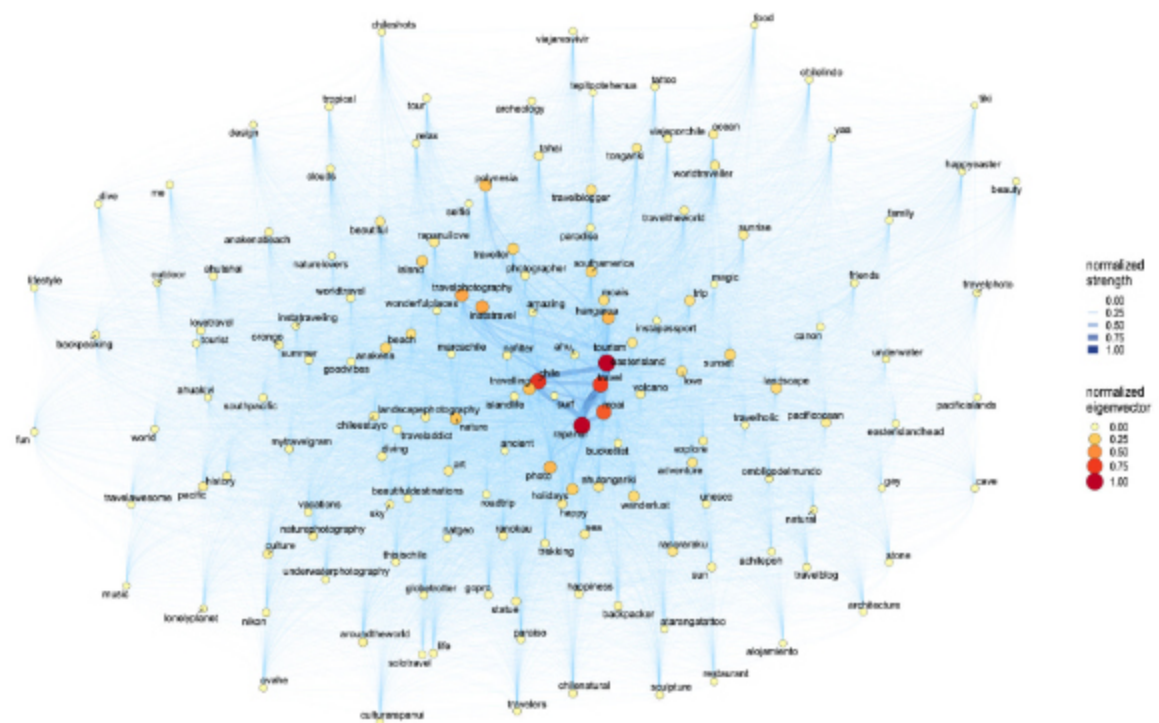

1B)

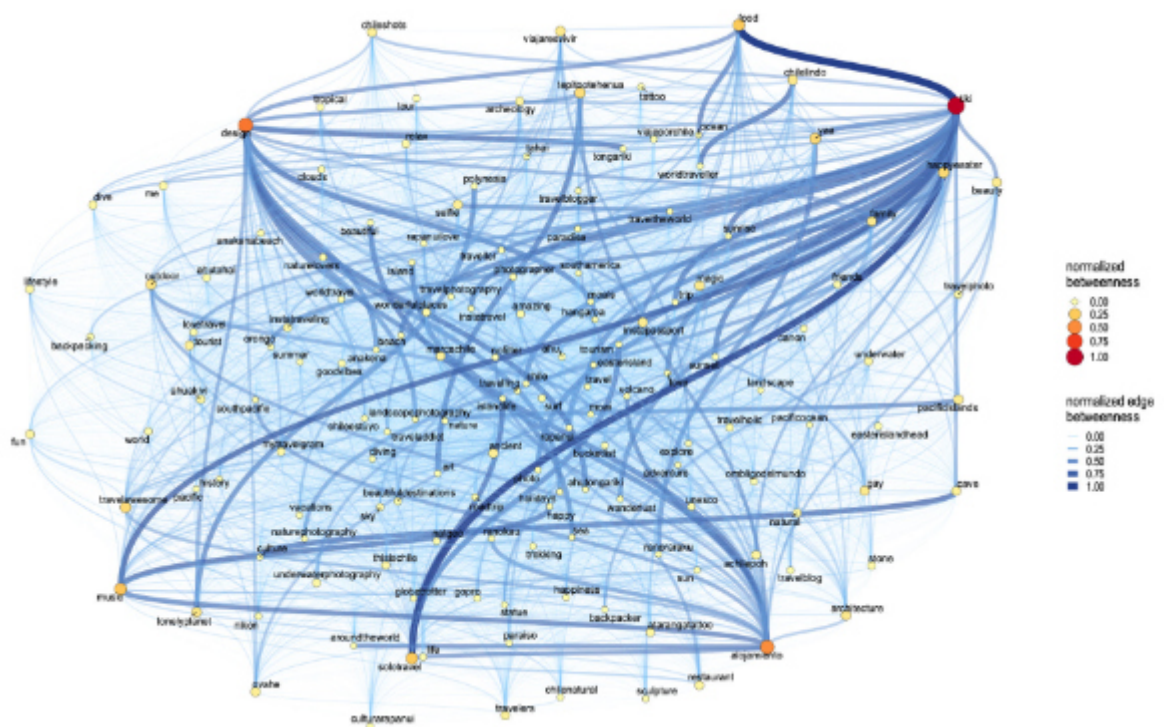

2A)

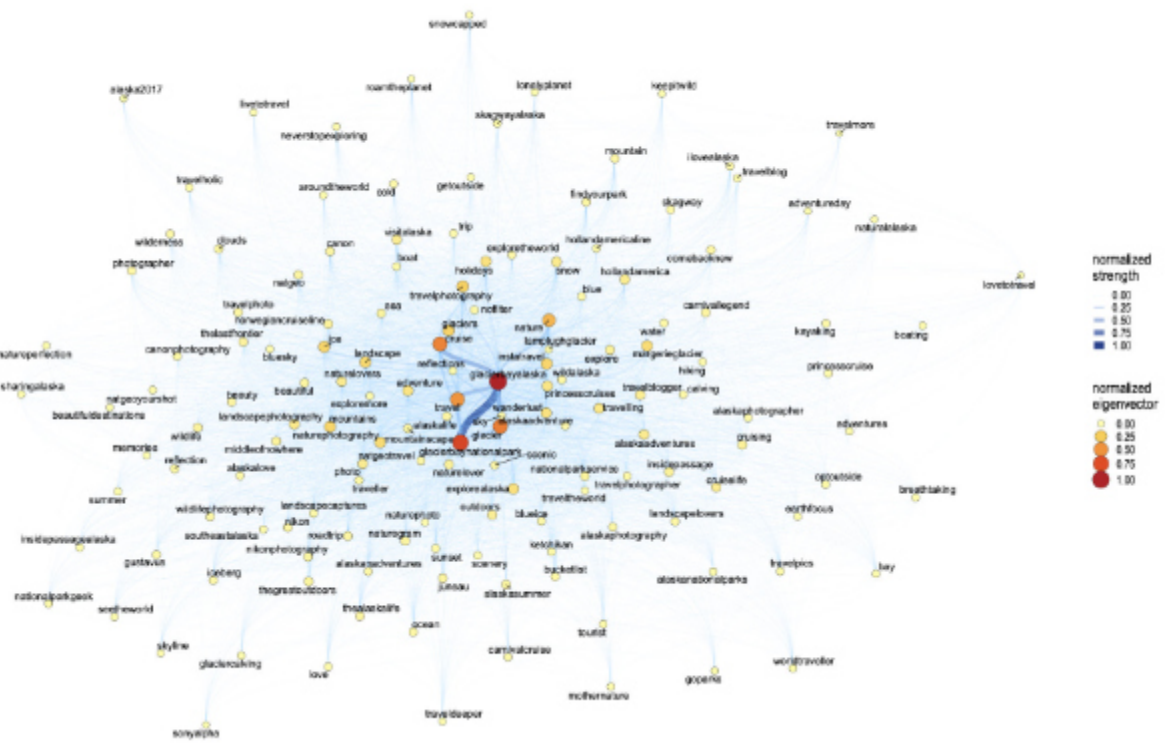

2B)

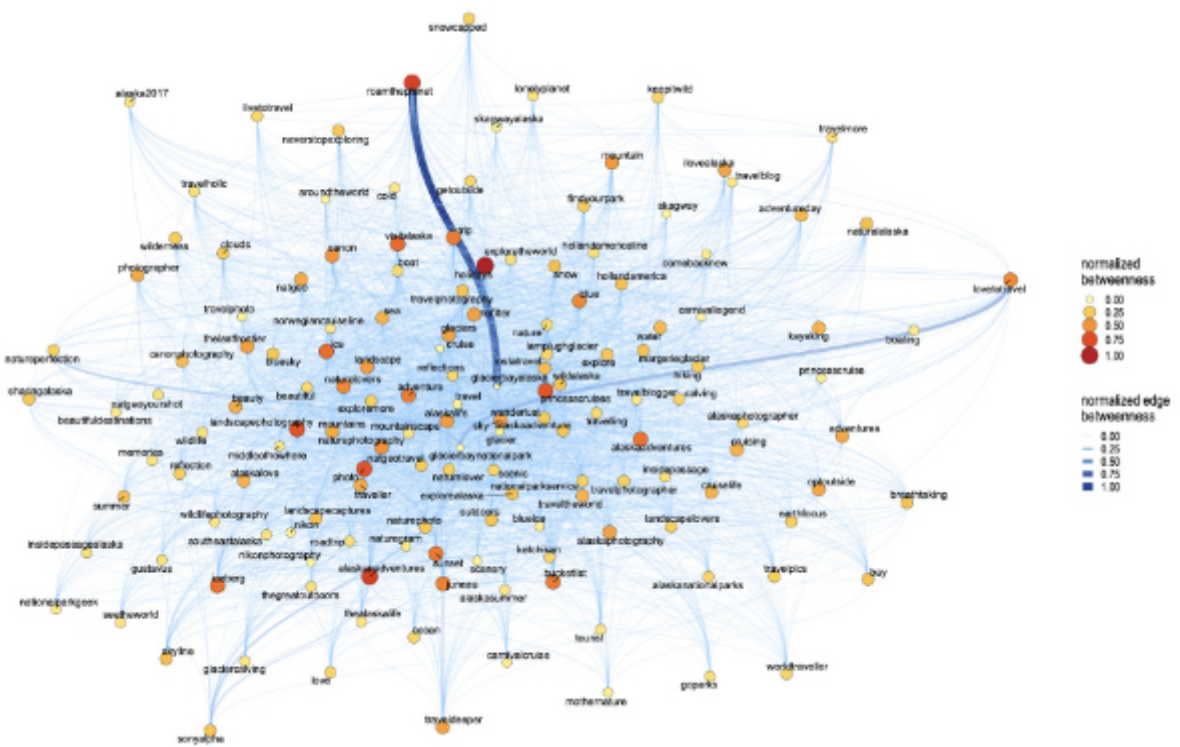

3A)

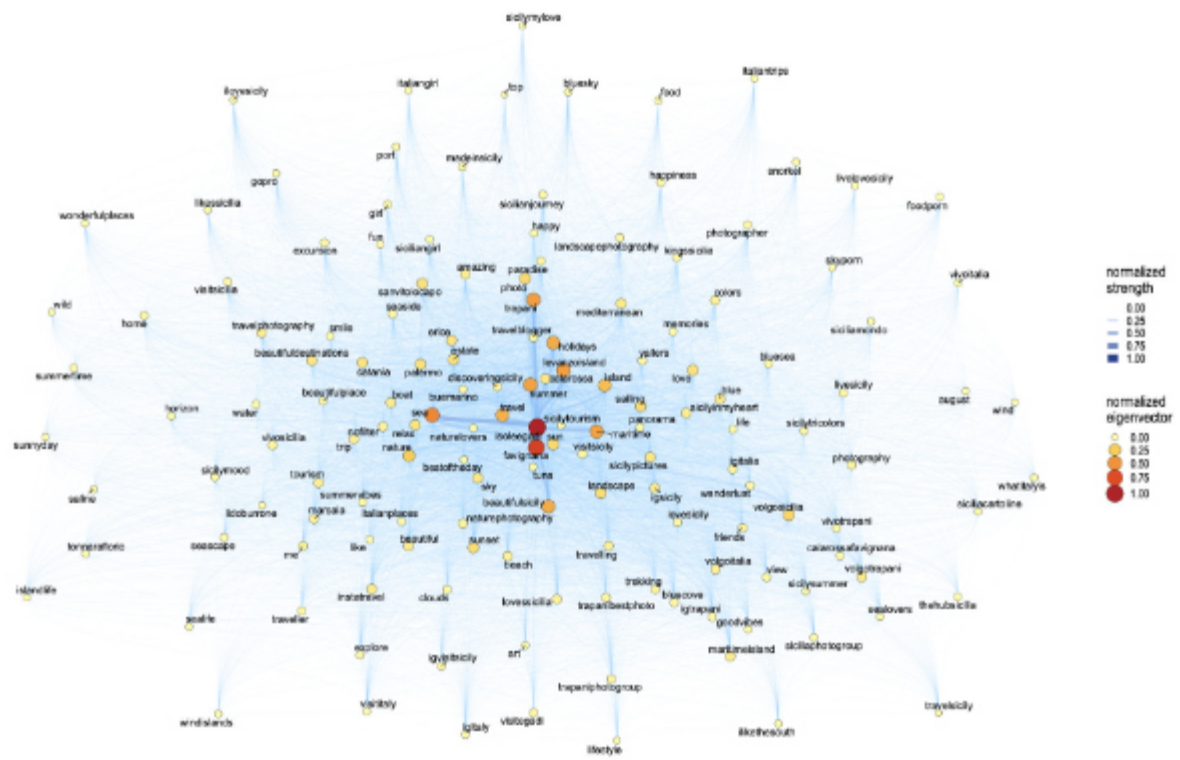

3B)

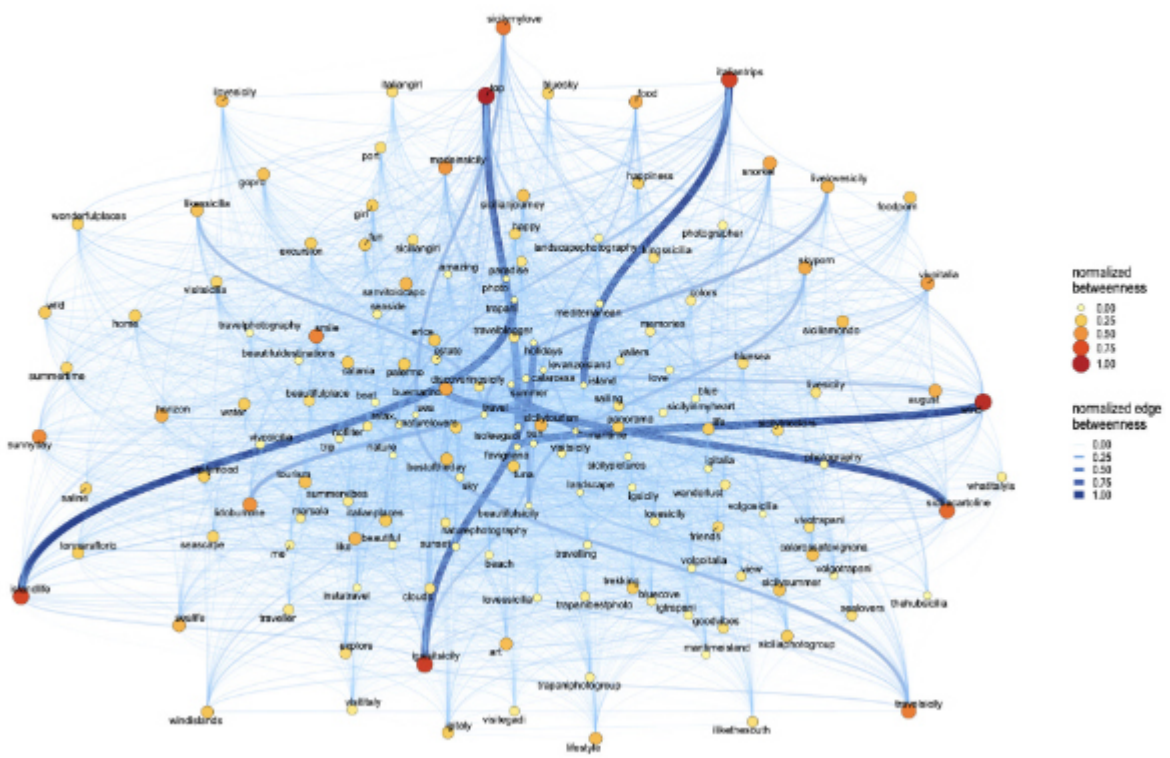

4A)

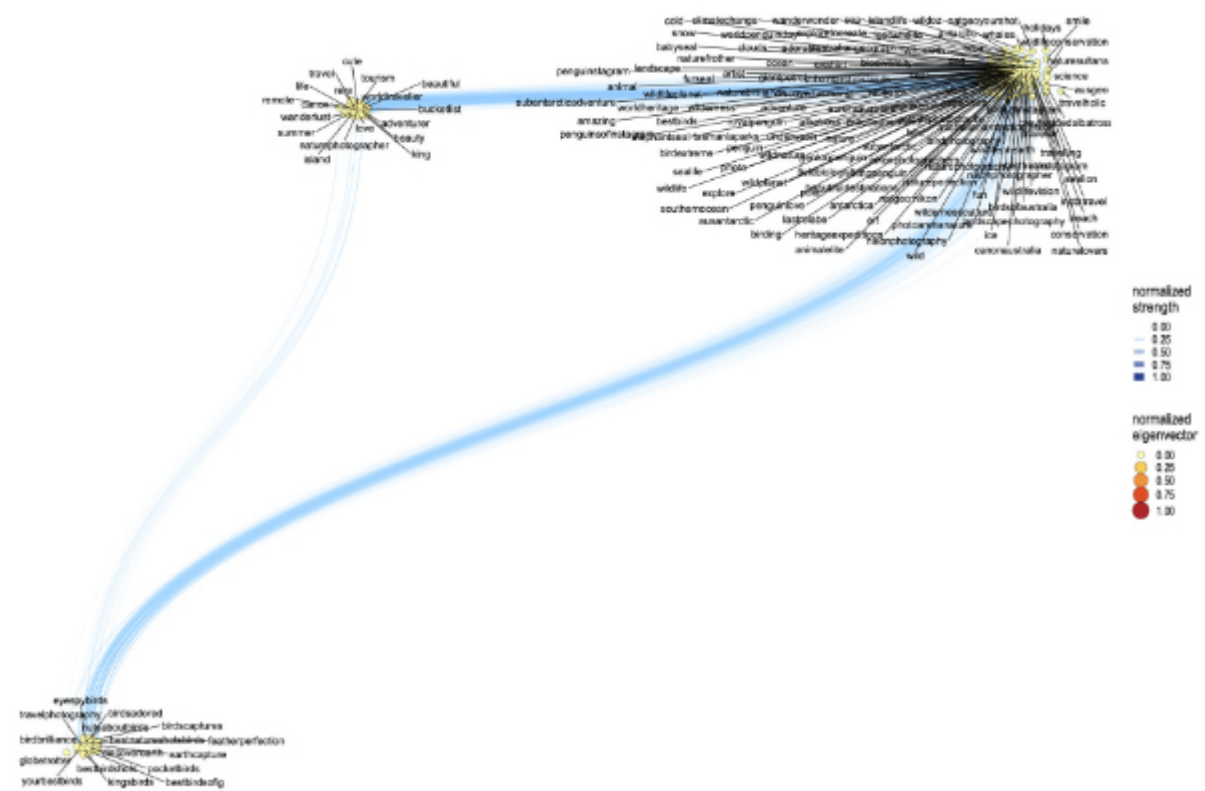

4B)

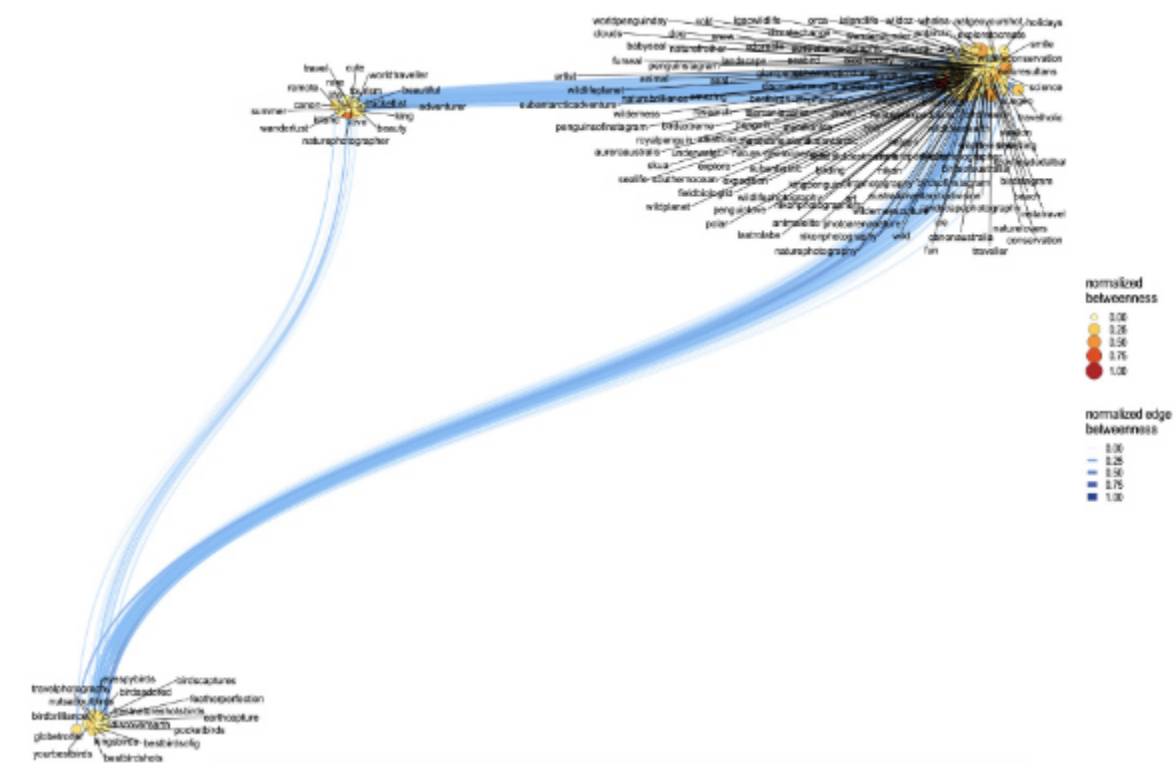

5A)

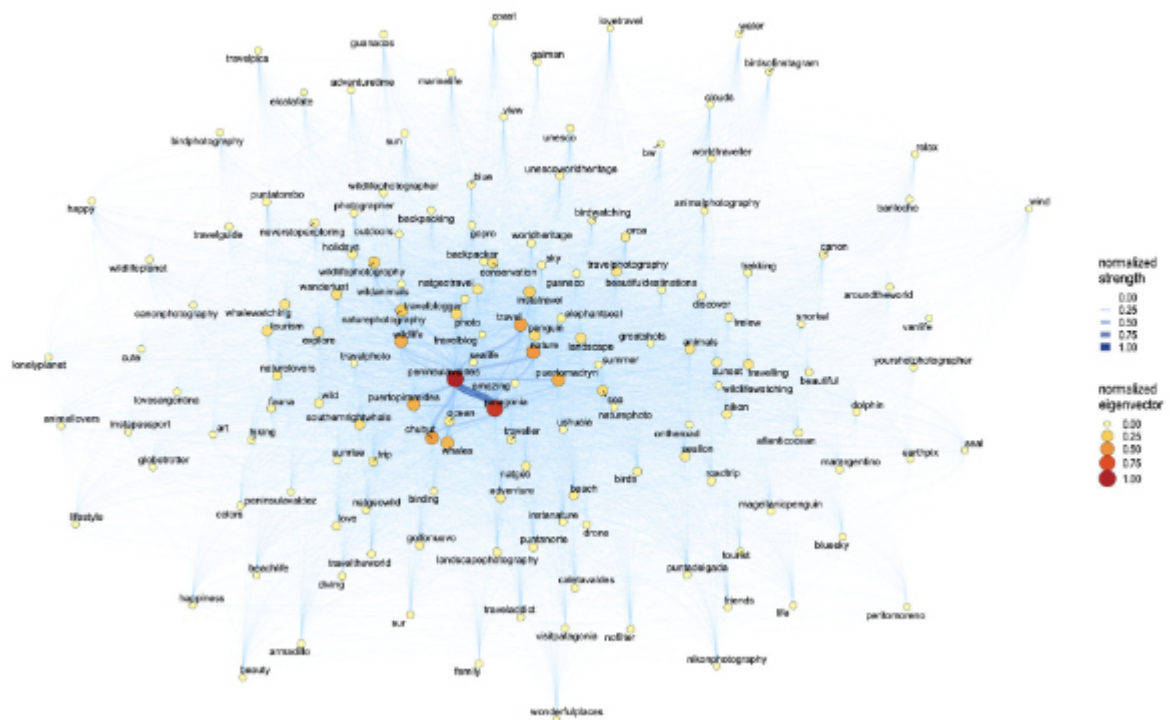

5B)

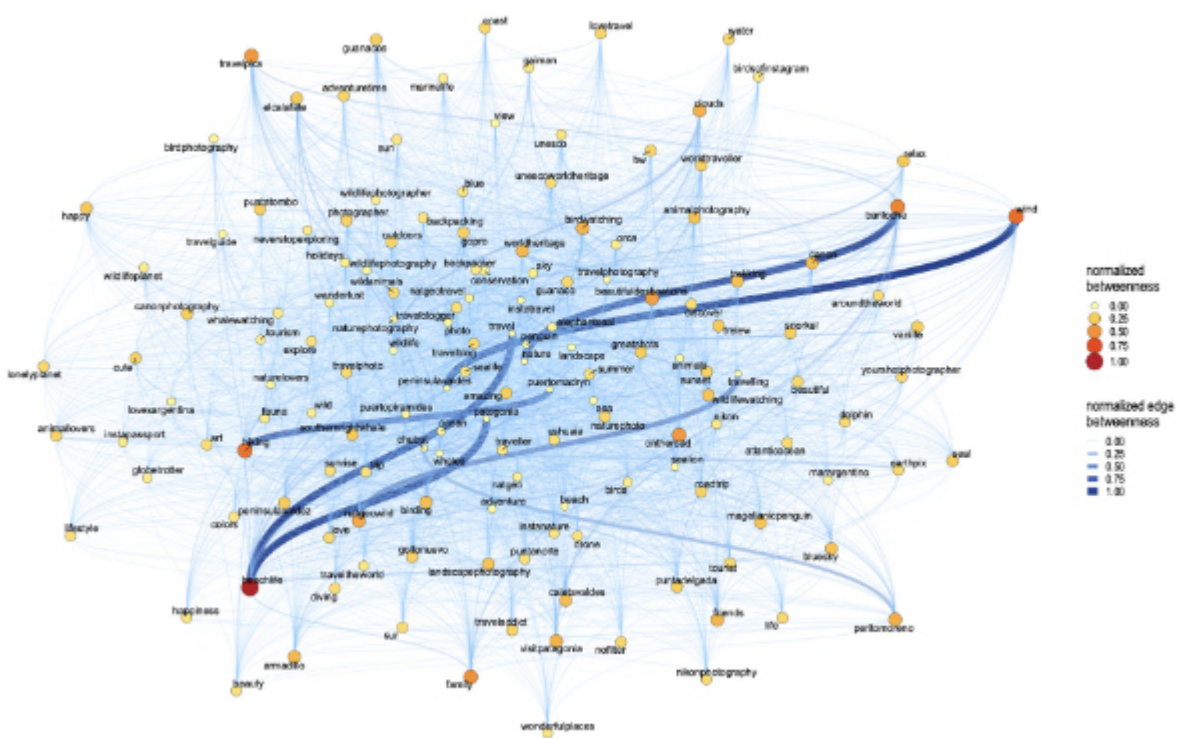

6A)

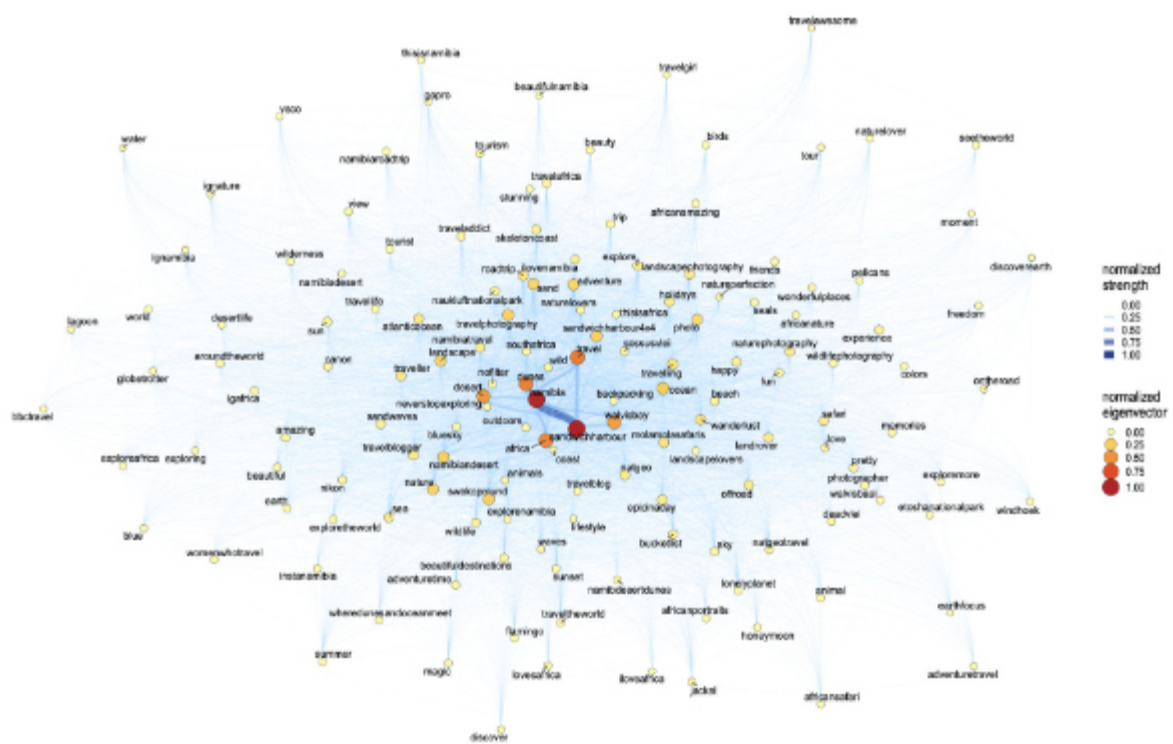

6B)

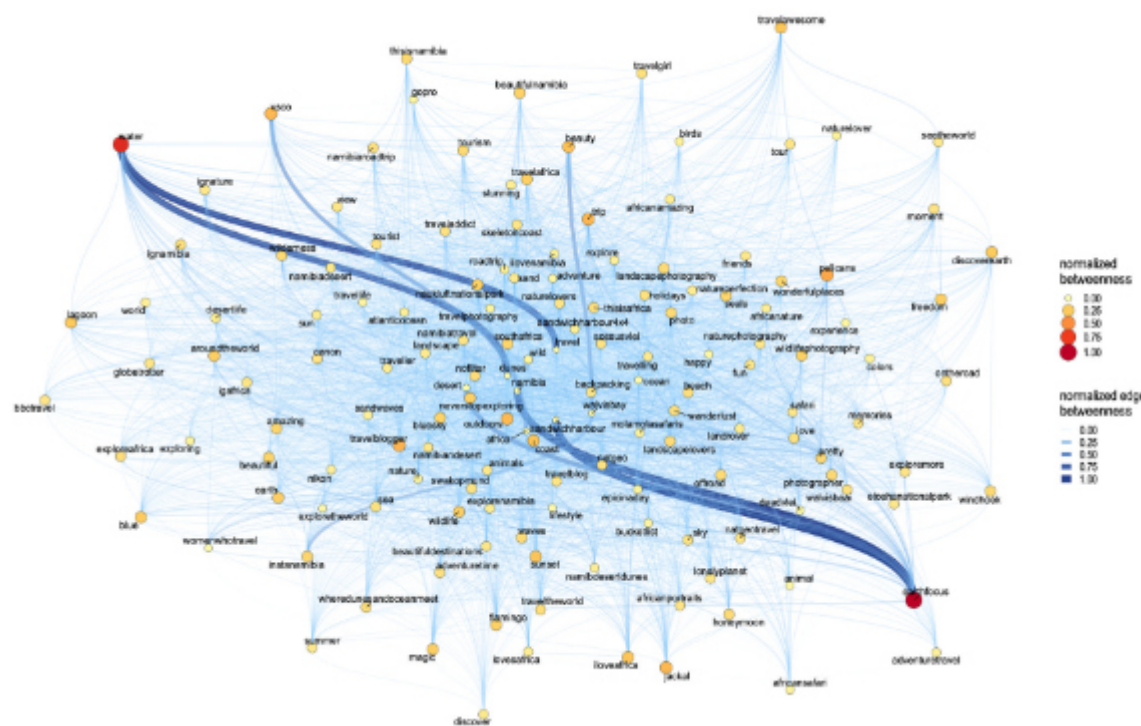

7A)

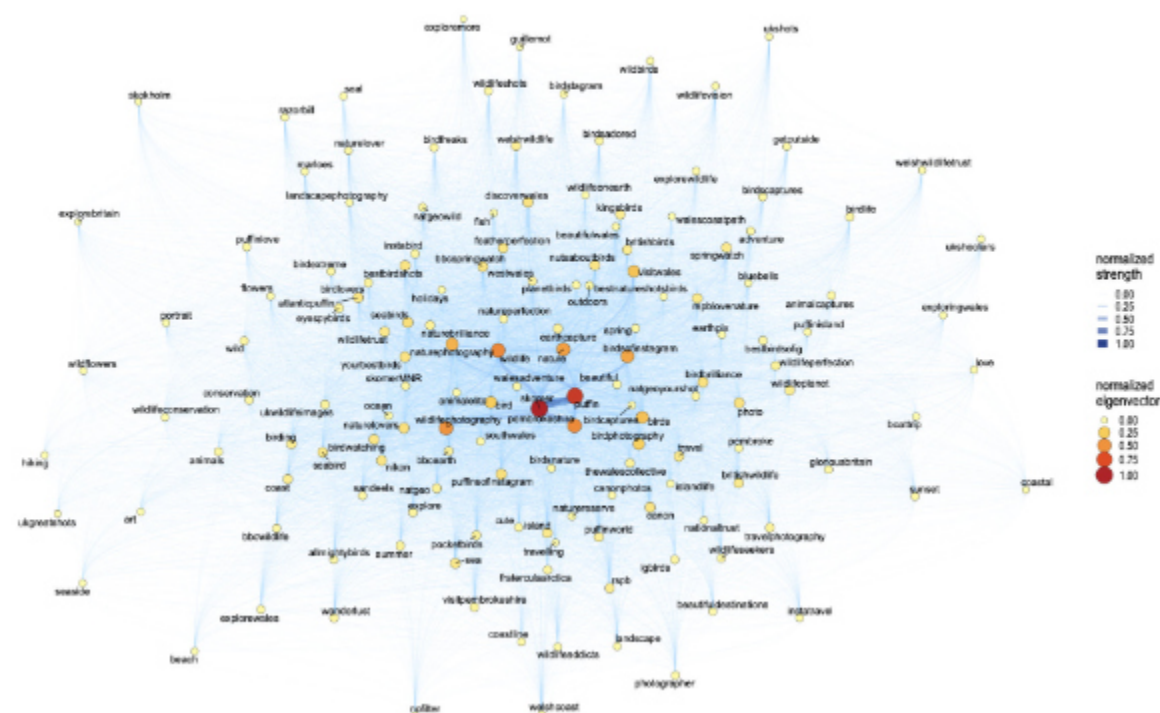

7B)

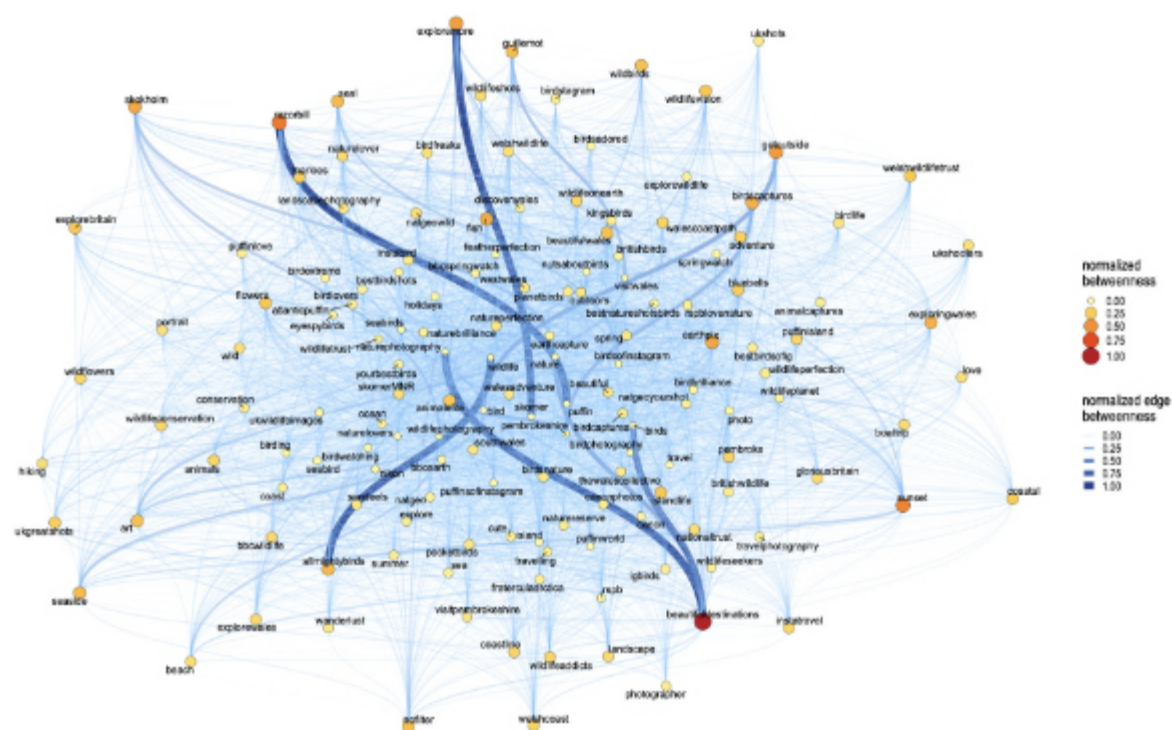

8A)

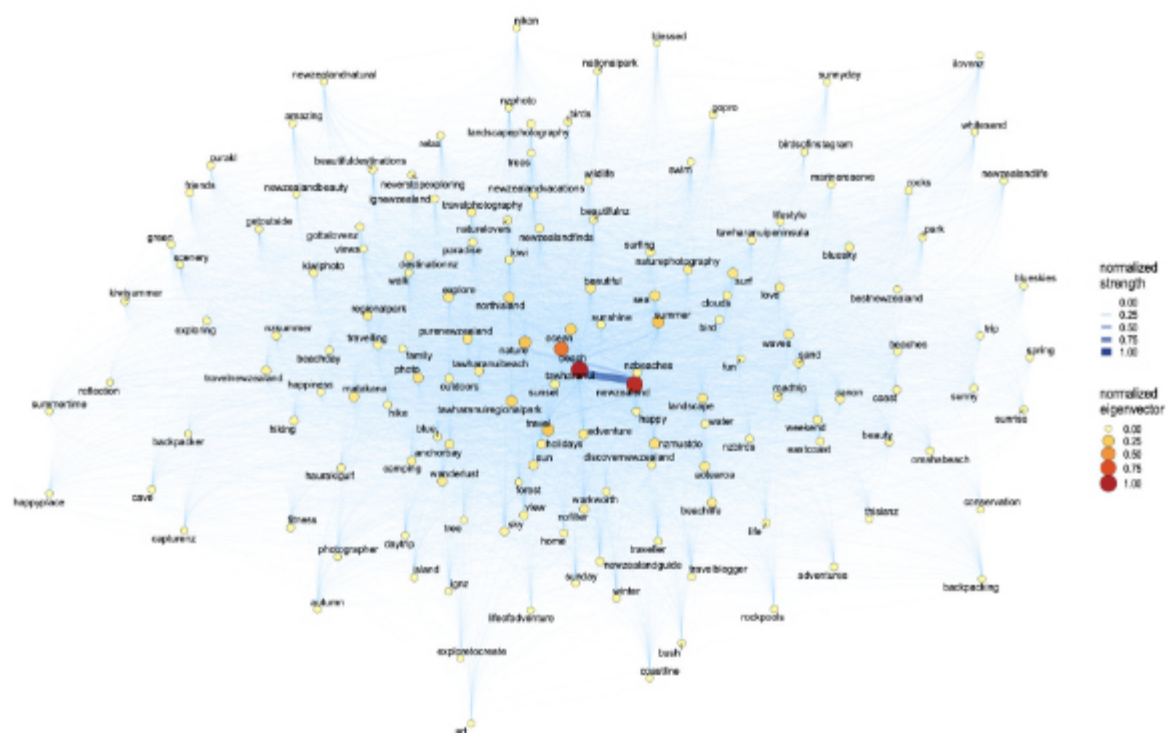

8B)

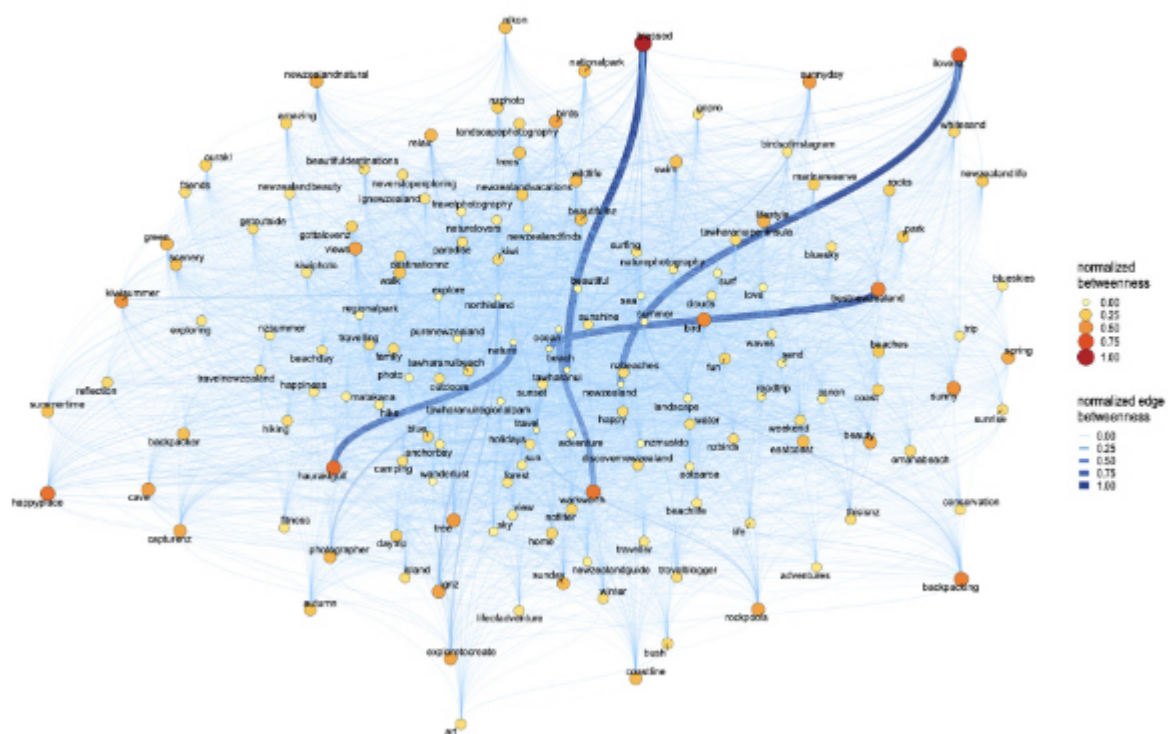

9A)

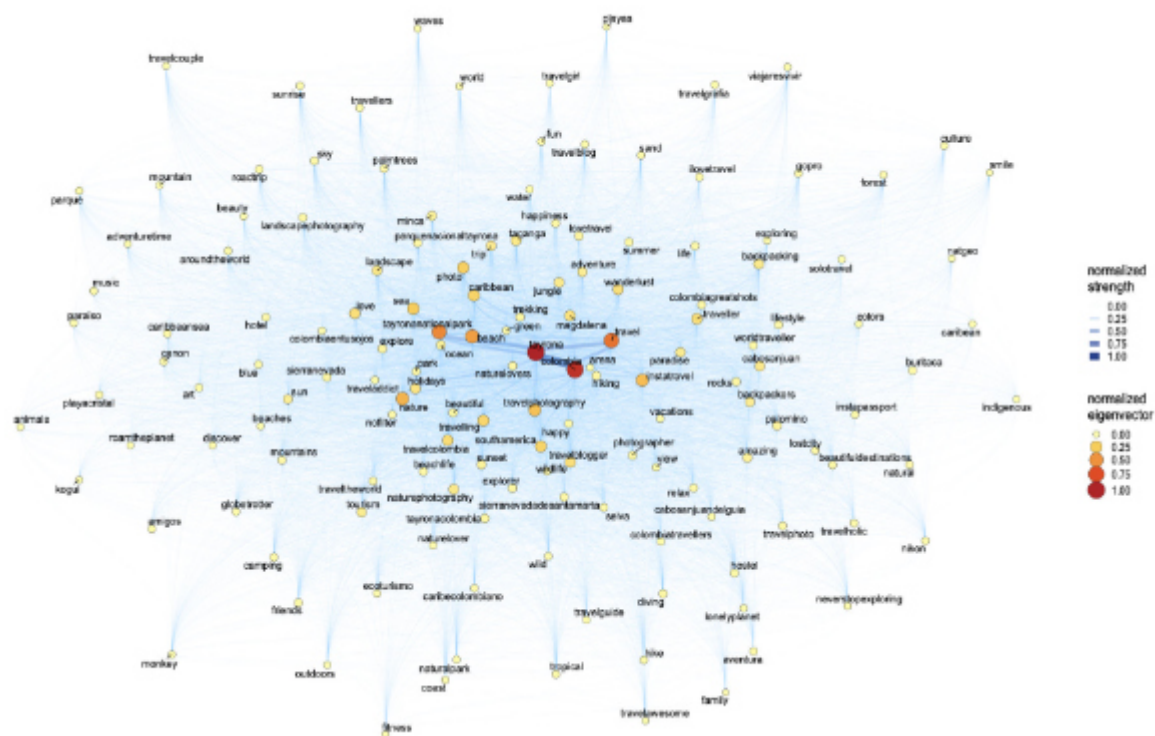

9B)



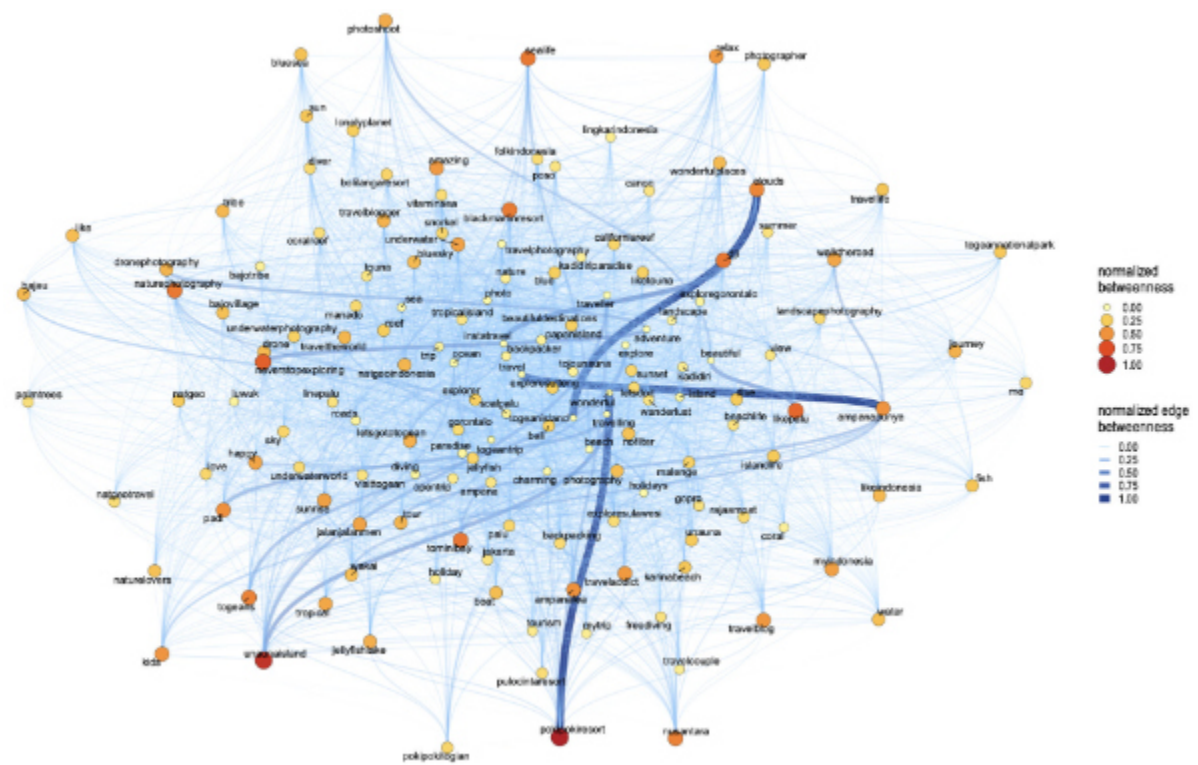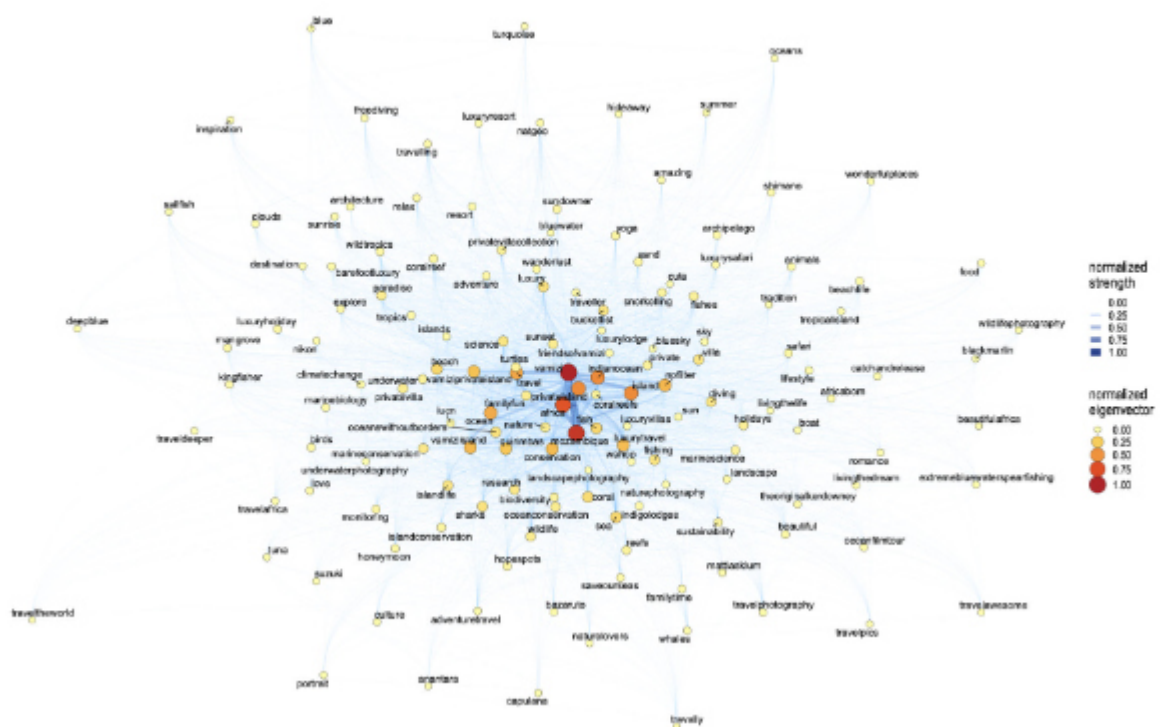

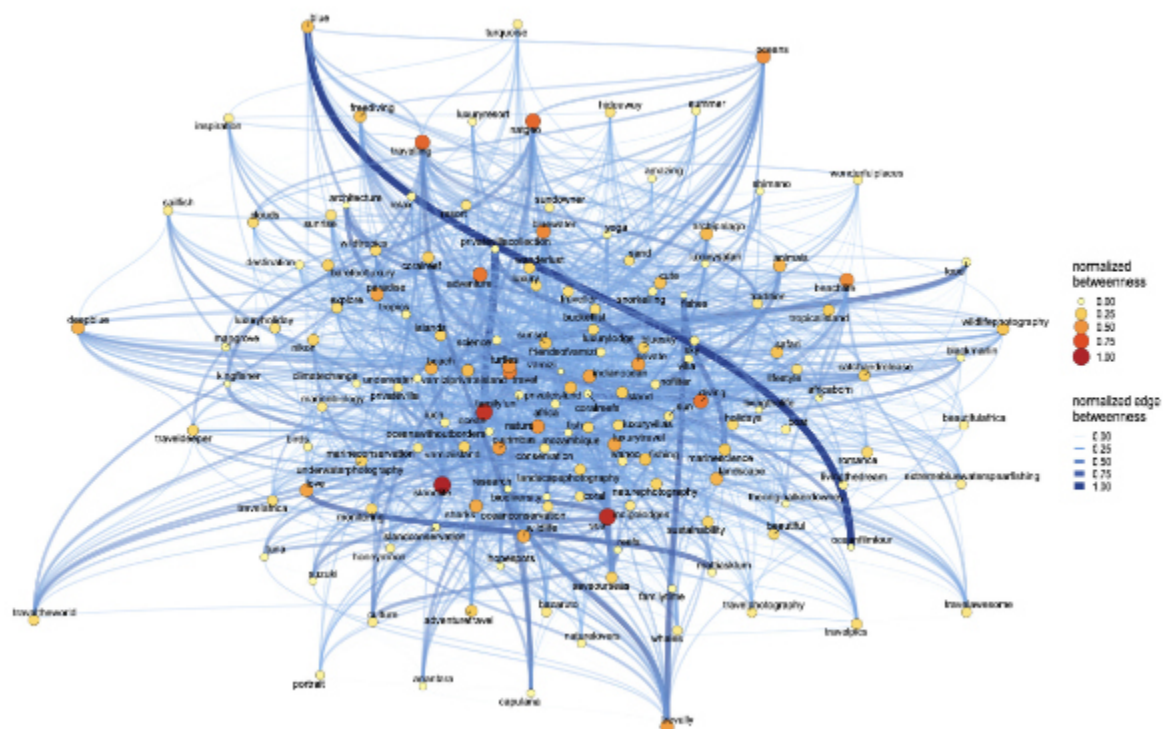

12A)

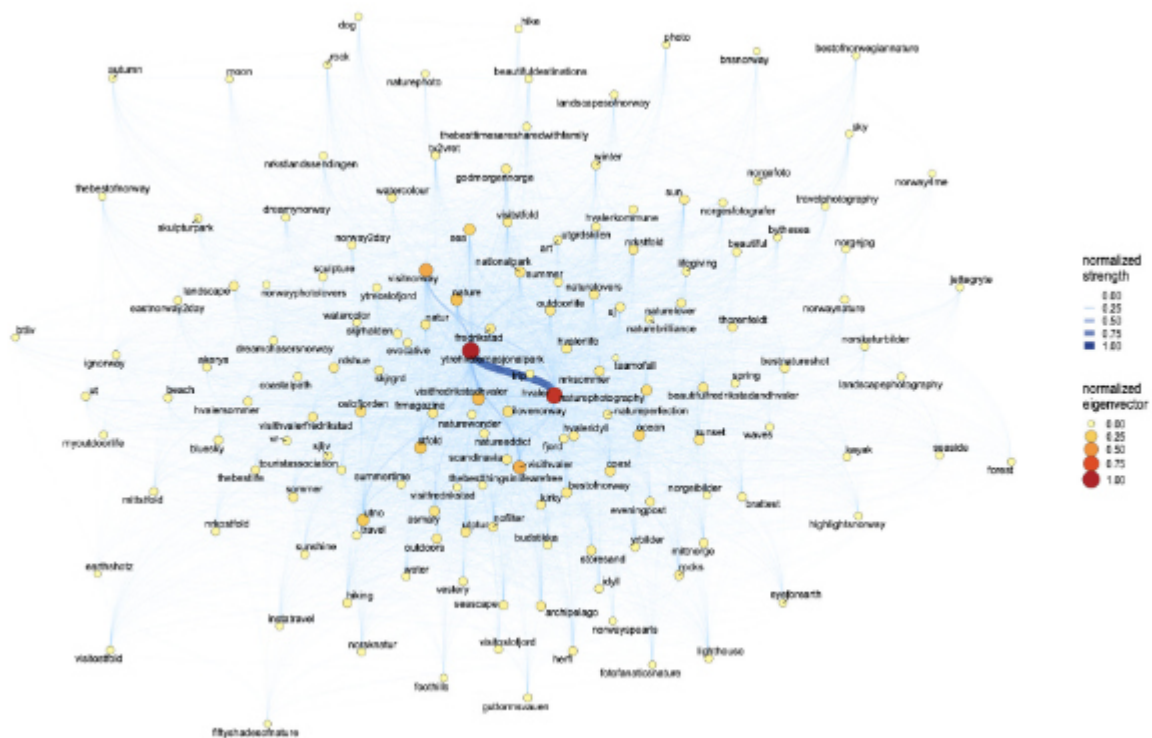

12B)

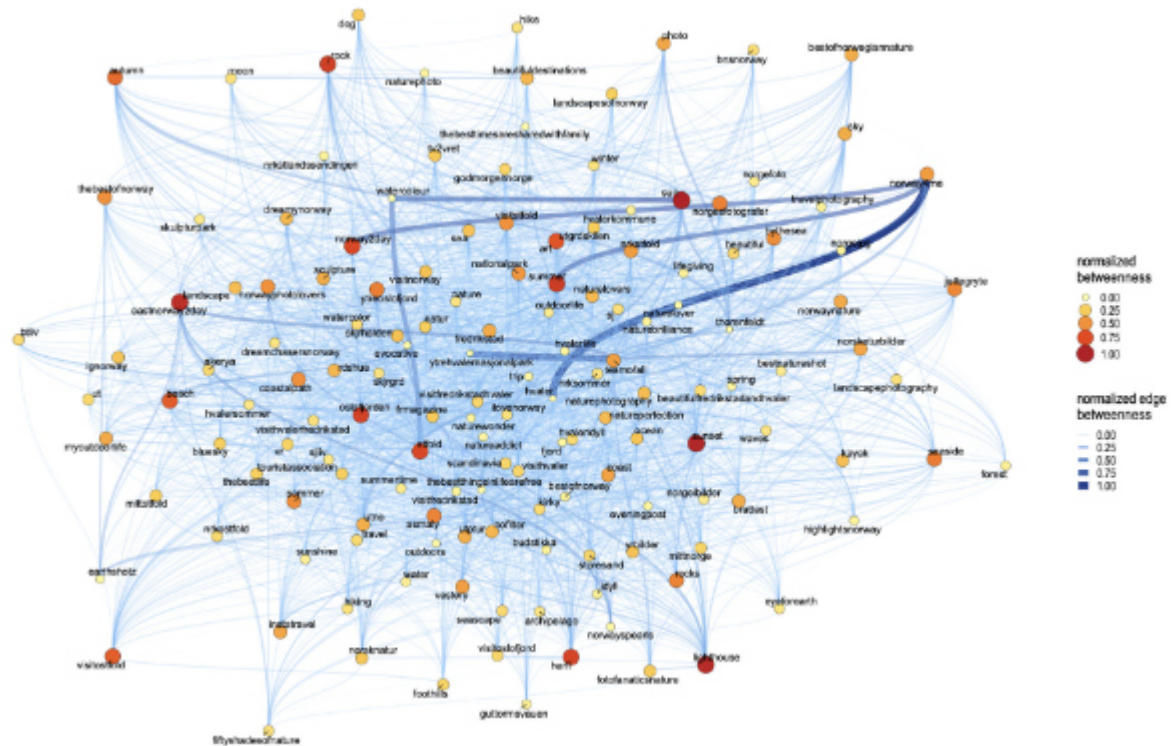

FIGURE A1 – Network graphs in the case studies: 1, Eastern Island; 2, Glacier Bay; 3, Isole Egadi; 4, Macquarie Island; 5, Peninsula Valdes; 6, Sandwich Harbour; 7, Skomer; 8, Tawharanui; 9, Tayrona; 10, Togean Island; 11, Vamizi; 12, Ytre Hvaler. A) represents the Eigenvector centrality, B) represents Betweenness centrality and Edge betweenness
