# Supplementary material for: A Graph Theory approach to assess nature's contribution to people at a global scale
Source: arXiv:2007.14308 source file (2021-02-15)
Supplement: Supplementary file 2 [file SI_FigA2_lowres.pdf]

## SUPPLEMENTARY MATERIAL

1)

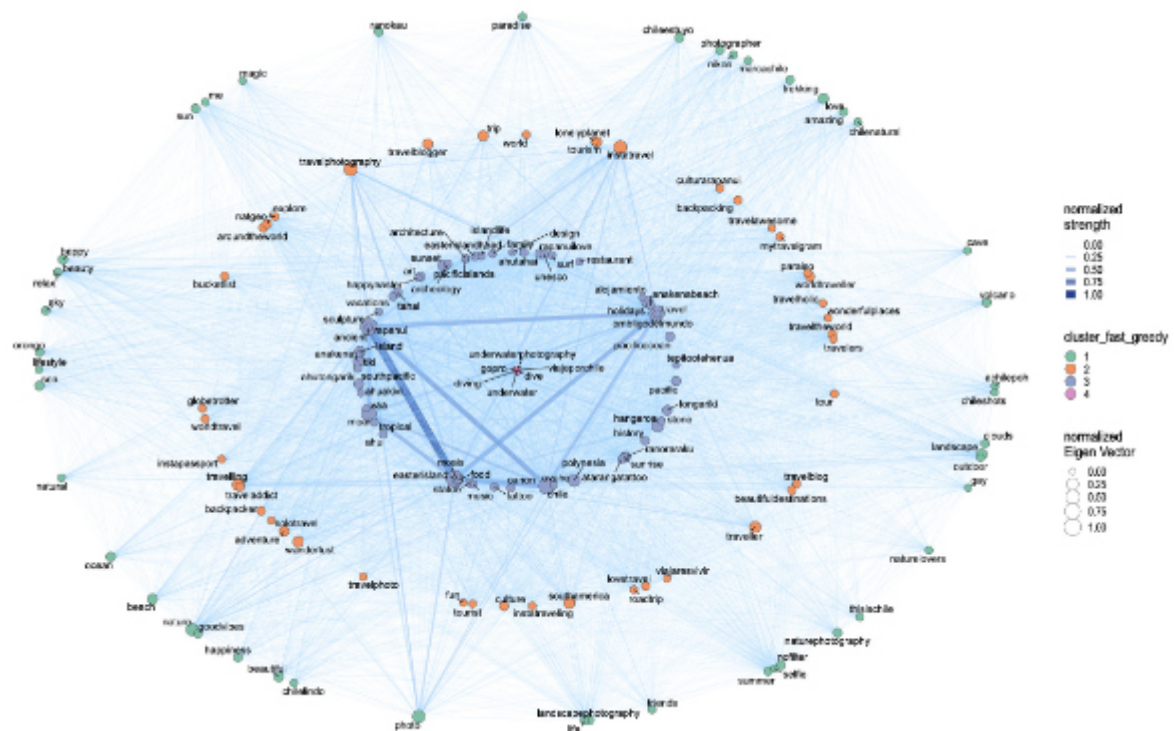

2)

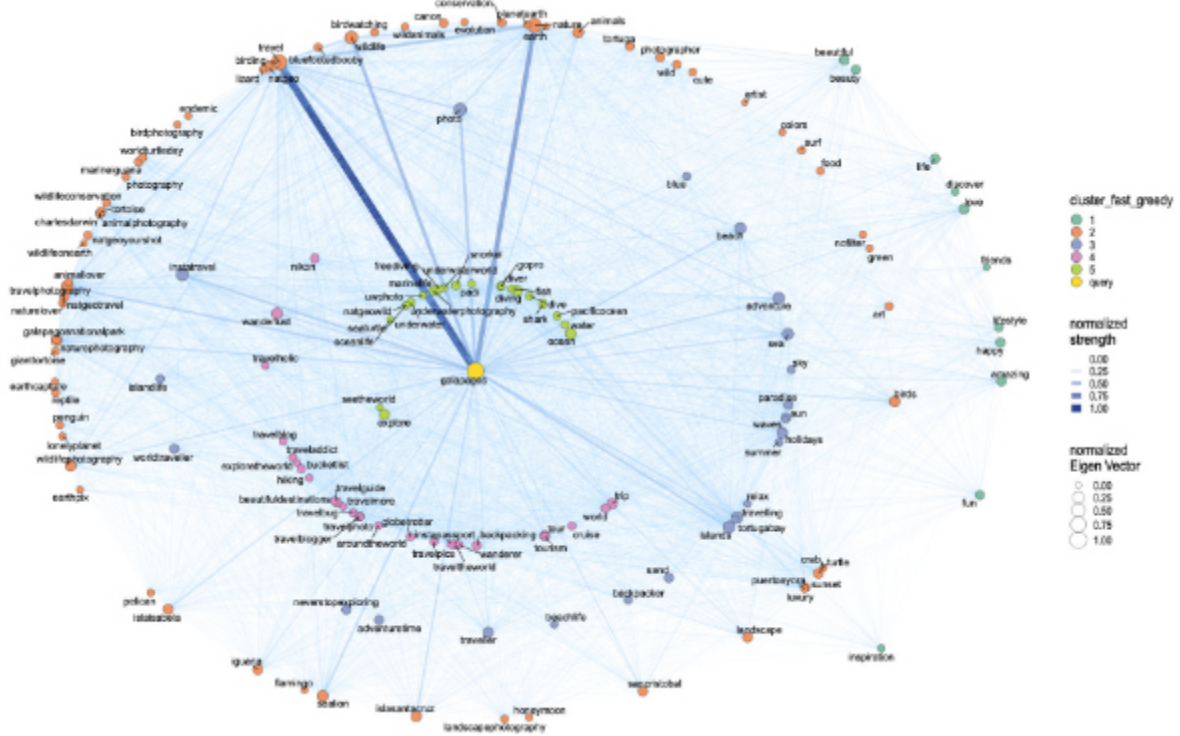

3)

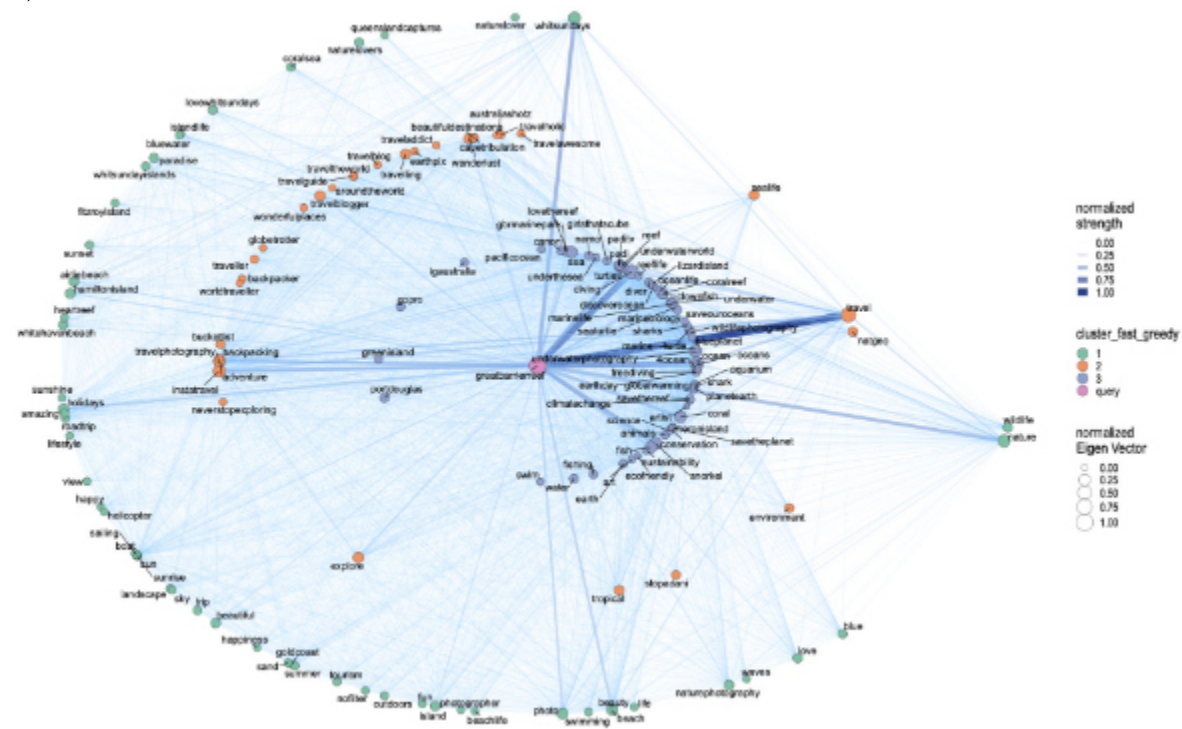

4)

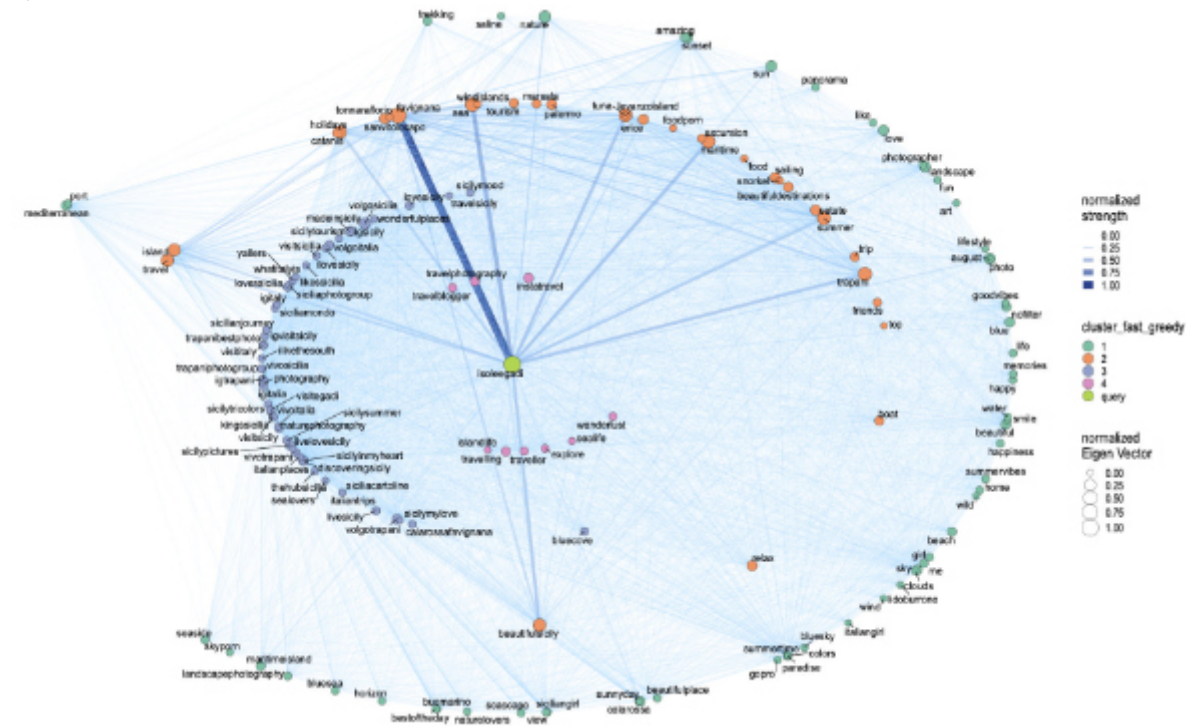



5)

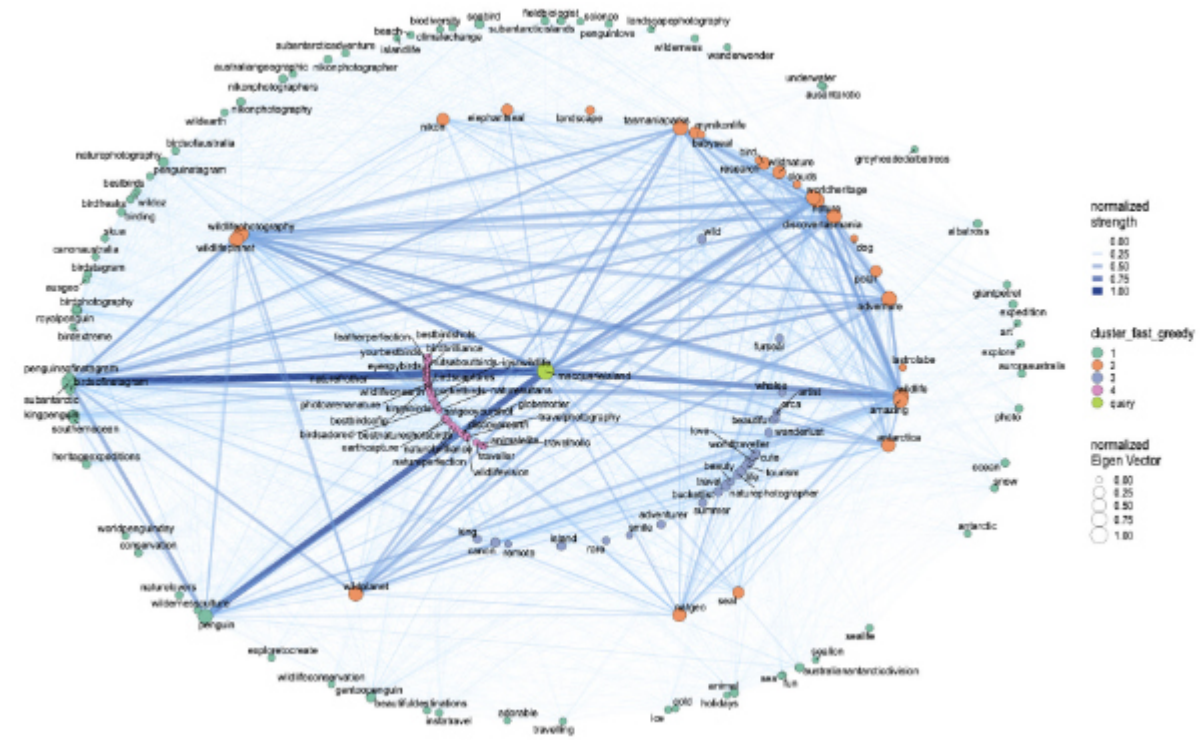

6)

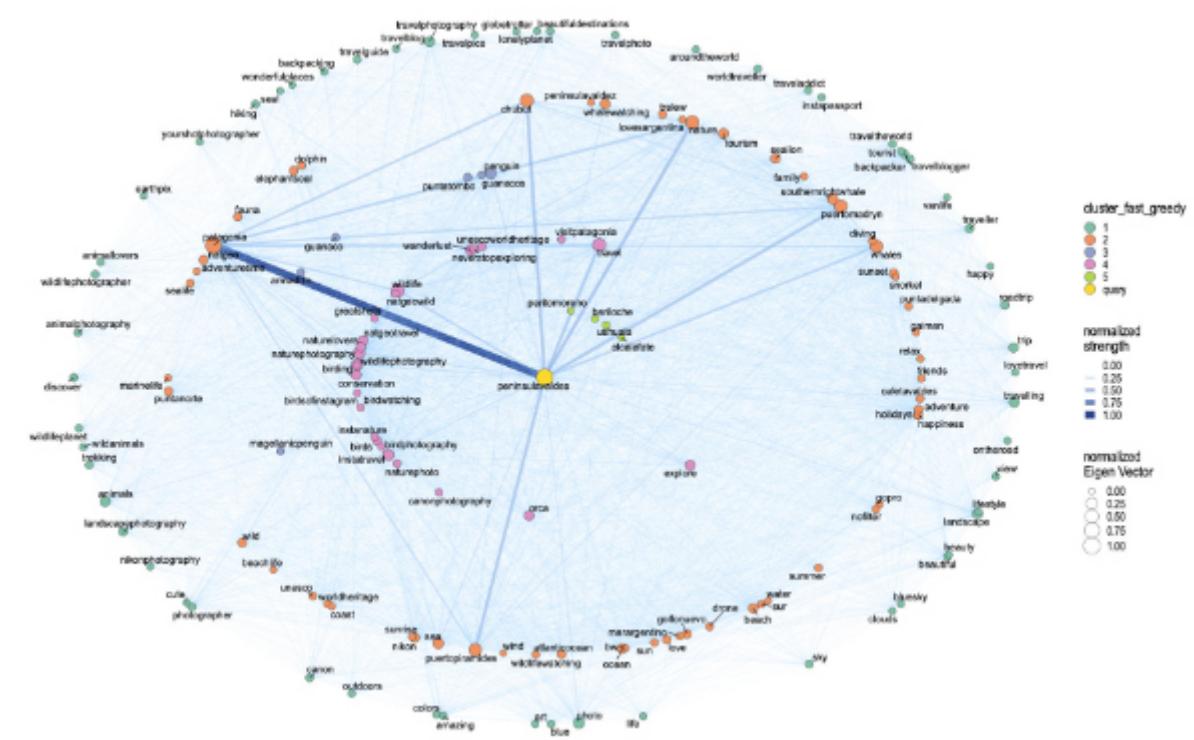

7)

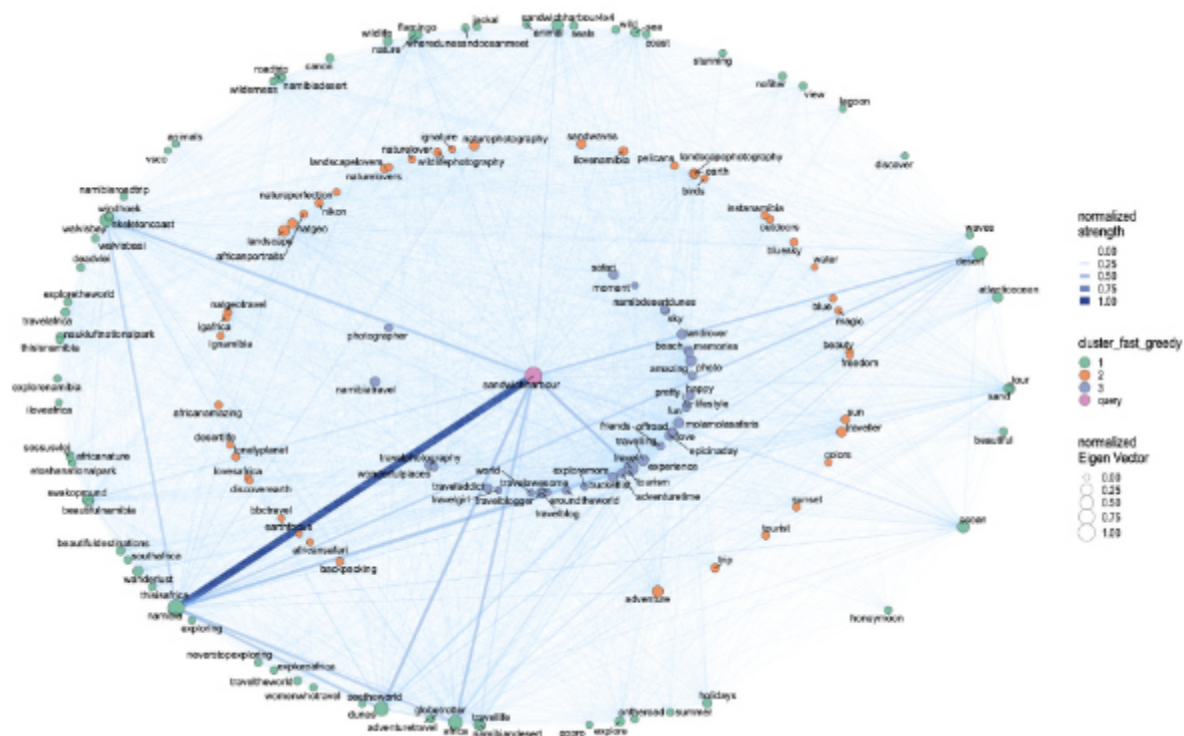

8)

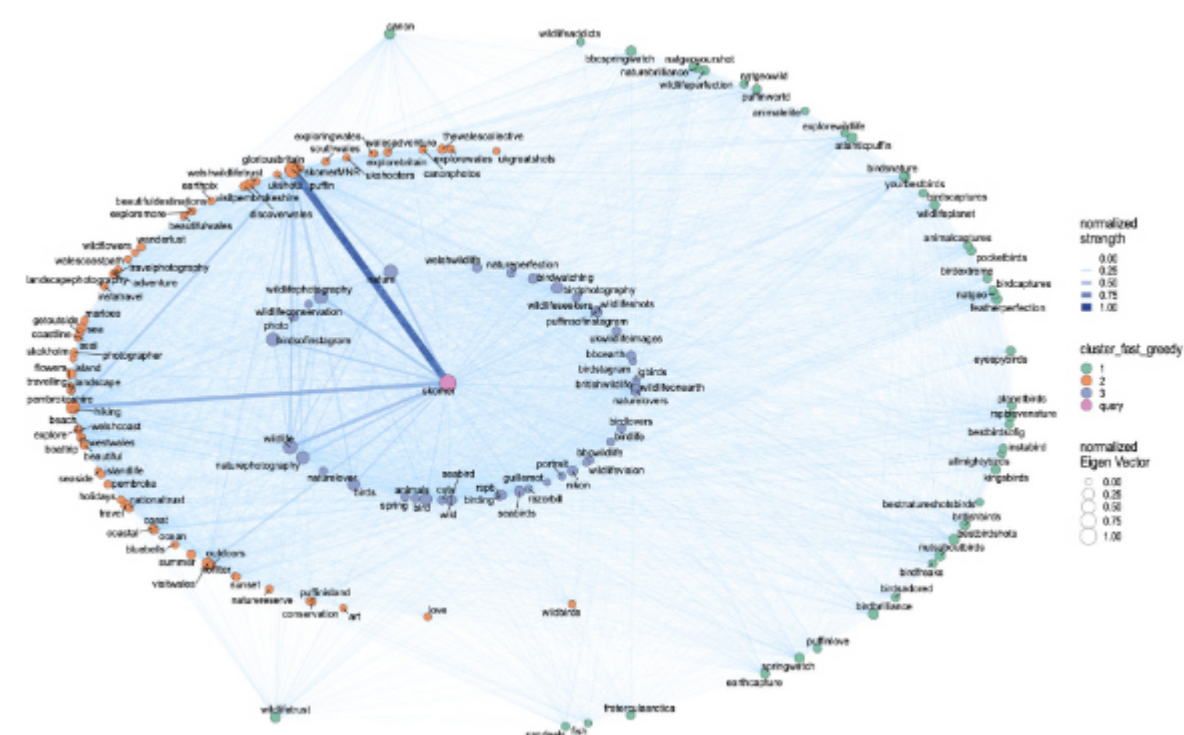



9)

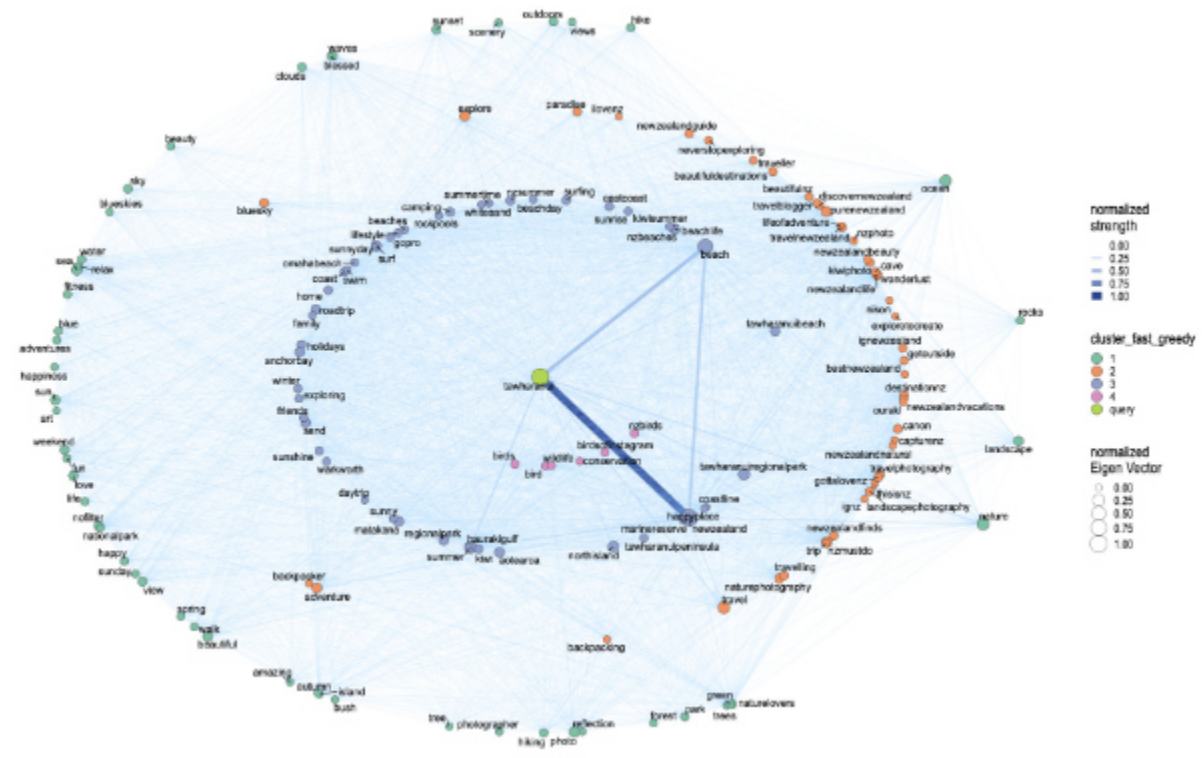

10)

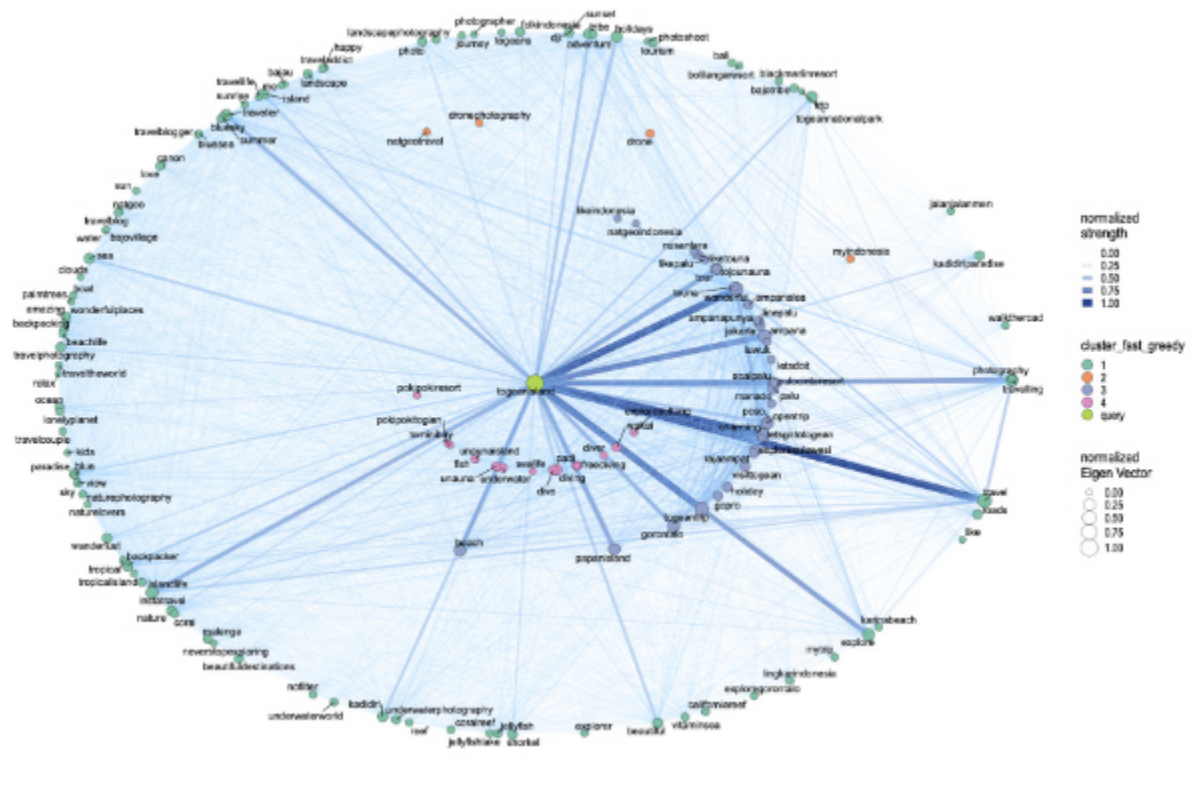

11)

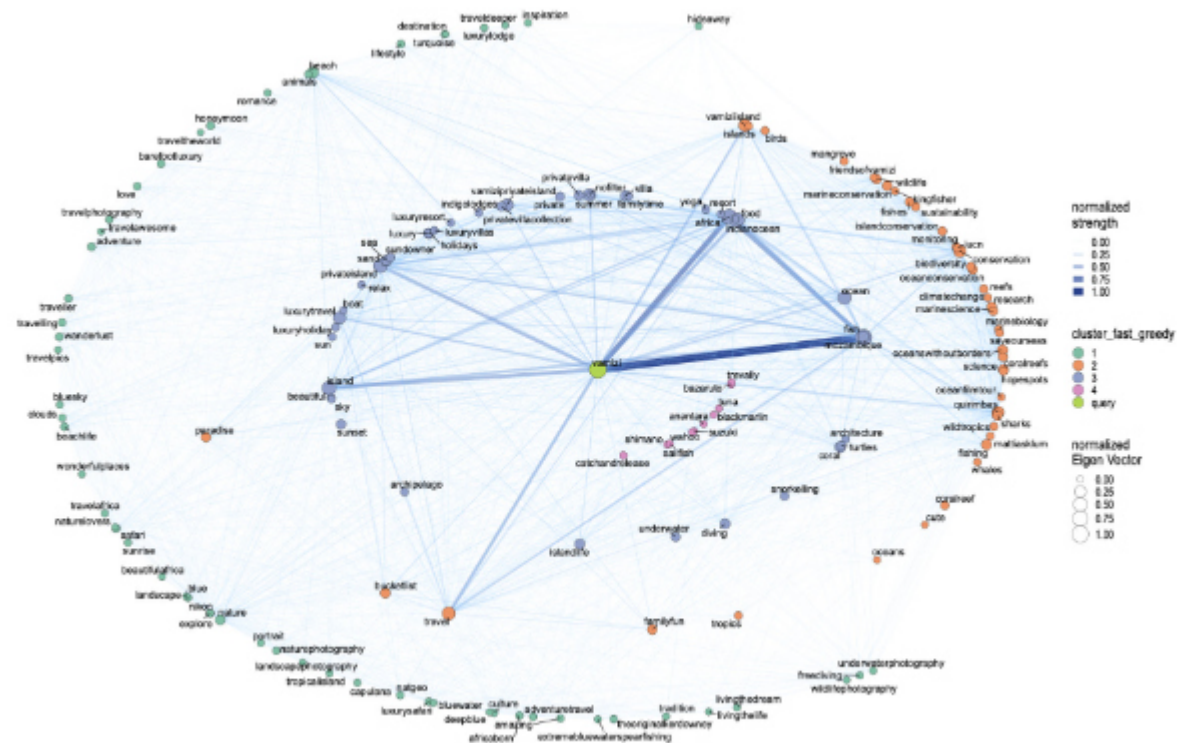

12)

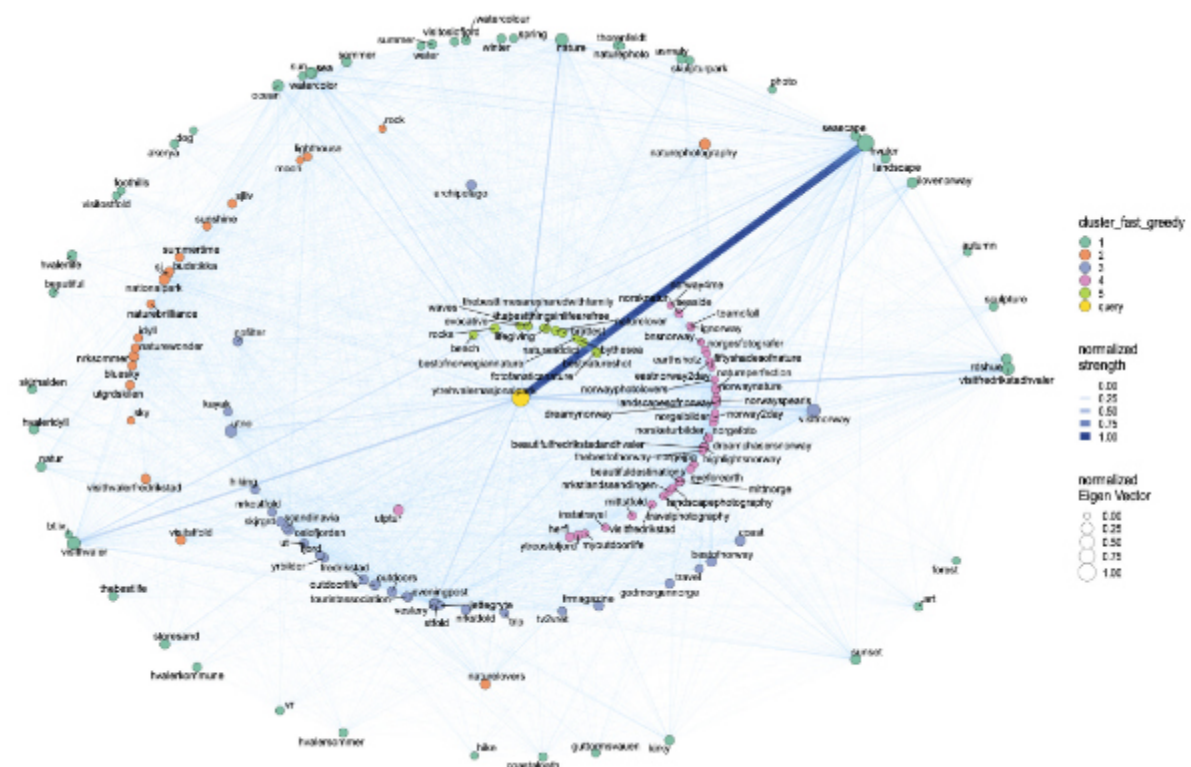

FIGURE A2 –Fast-Greedy community algorithm for the case studies: 1, Eastern Island; 2, Galapagos; 3, Great Barrier Reef; 4, Isole Egadi; 5, Macquarie Island; 6, Peninsula Valdes; 7, Sandwich Harbour; 8, Skomer; 9, Tawharanui; 10, Togean Island; 11, Vamizi; 12, Ytre Hvaler
